# Supplementary material for: SoccerNet-Caption: Dense Video Captioning for Soccer Broadcasts Commentaries
Source: arXiv:2304.04565 source file (2023-04-10)
Supplement: Supplementary file 1 [file supplementary.tex]

\begin{figure}[t]
    \includegraphics[width=\linewidth]{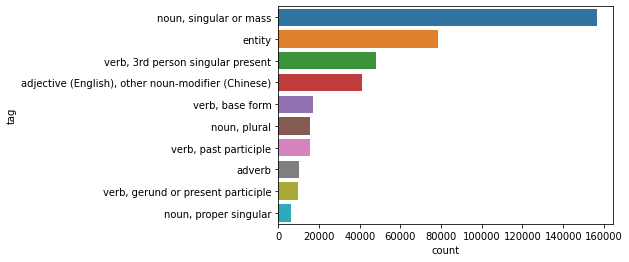}
    \caption{Test1}
    \label{fig:}
\end{figure}

\begin{figure}[t]
    \includegraphics[width=\linewidth]{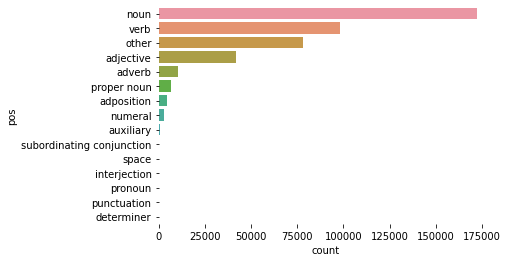}
    \caption{Test3}
    \label{fig:pulling}
\end{figure}

\begin{figure}[t]
    \includegraphics[width=\linewidth]{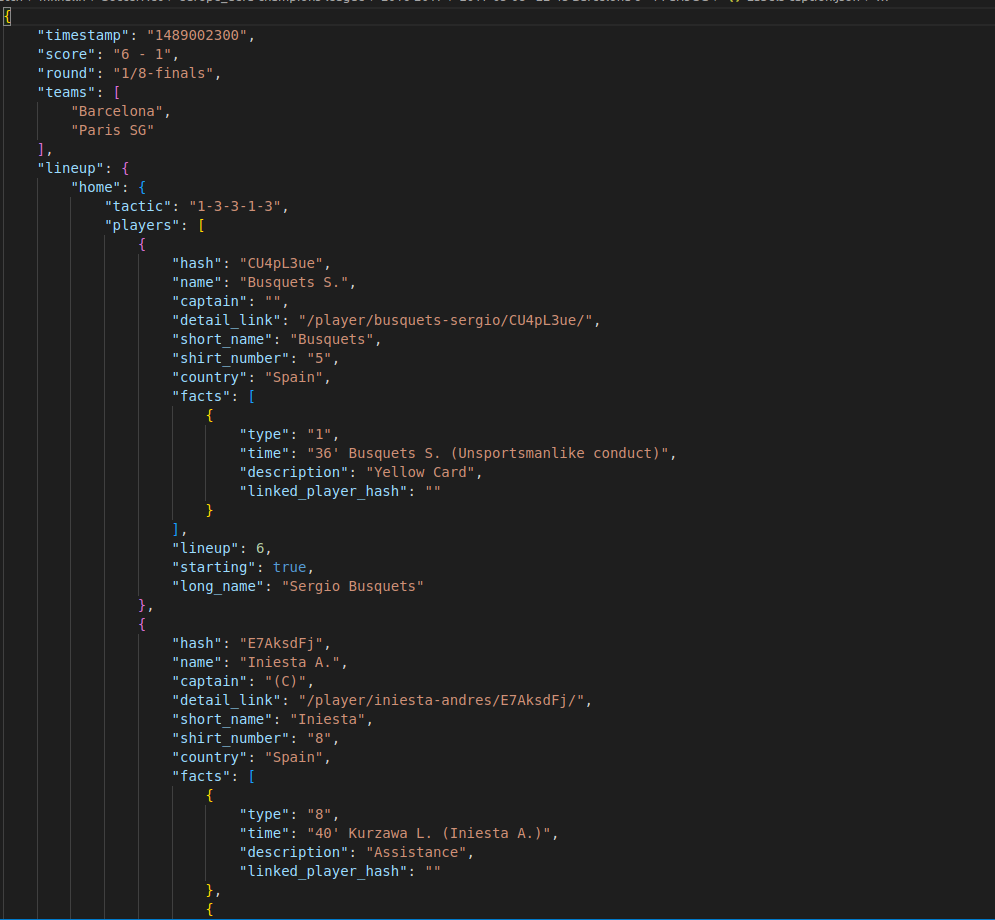}
    \caption{Test3}
    \label{fig:pulling}
\end{figure}

\begin{figure}[t]
    \includegraphics[width=\linewidth]{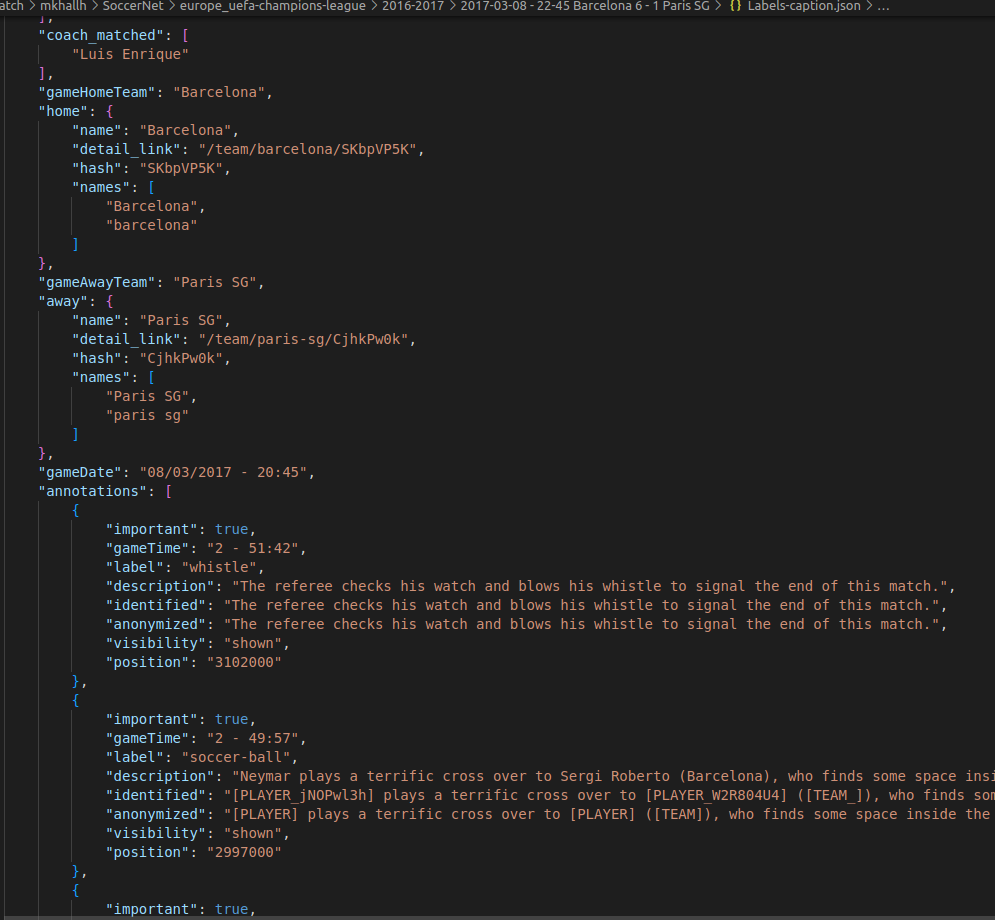}
    \caption{Test3}
    \label{fig:pulling}
\end{figure}
